# Supplementary material for: Prune 'n Predict: Optimizing LLM Decision-making with Conformal Prediction
Source: arXiv:2501.00555 source file (2025-07-12)
Supplement: Supplementary file 1 [file accuracy_derivations.tex]

\section{Accuracy Derivations [remove for submission]}

What factors cause the accuracy to go up with CROQ?

For a given MCQ, let:
\begin{align*}
    B &= 1\{\text{LLM is correct before CROQ}\} && \text{``before''} \\
    R &= 1\{\text{The CP prediction set contains the correct answer}\} && \text{``retains''} \\
    A &= 1\{\text{The LLM is correct after CROQ}\} && \text{``after''}
\end{align*}
where $1\{\cdot\}$ is the indicator function. Then the accuracy before CROQ is $\E[B] = \Pb(B = 1)$, and the accuracy after CROQ is $\E[A] = \Pb(A = 1)$. Can we come up with any insight as to when $\E[A] > \E[B]$?

We have:
\begin{align}
    \E[A] &= \E[\E[A \mid B, R]] \\
          &= \E[A \mid B = 0, R = 1]\Pb(B = 0, R = 1) + \E[A \mid B = 1, R = 1]\Pb(B = 1, R = 1) \\
          &= \E[A \mid B = 0, R = 1]\Pb(R = 1 \mid B = 0)\Pb(B = 0) + \E[A \mid B = 1, R = 1]\Pb(R = 1 \mid B = 1)\Pb(B = 1) \\
          &= \E[A \mid B = 0, R = 1]\Pb(R = 1 \mid B = 0)(1 - \Pb(B = 1)) + \E[A \mid B = 1, R = 1]\Pb(R = 1 \mid B = 1)\Pb(B = 1)  \label{eq:accuracy_derivation1}
\end{align}
where the first line uses the law of iterated expectation and the second line follows from the fact that $R = 0 \implies A = 0$.

Here are some assumptions/tools we could use for further derivations:
\begin{enumerate}
    \item $R$ is positively correlated with $B$, from which it follows that $\Pb(R = 1 \mid B = 0) < 1 - \alpha < \Pb(R = 1 \mid B = 1)$. This should be true in general.
    \item In fact, with logits as the scores, if we implicitly condition on the conformal sets being non-empty, then we have $\Pb(R = 1 \mid B = 1) = 1$, since $B = 1$ means the correct answer has the highest score, so it has to be included in any non-empty set. Conditioning on non-empty sets makes sense, because if we get an empty set, we just revert to the LLM's original answer.
    \item We can probably assume $\E[A \mid R = 1, B = 1] \geq \E[A \mid R = 1, B = 0]$. That is, if the LLM was correct before CROQ and the correct answer is retained, then it's highly likely to be correct after CROQ. It's somewhat less likely for the LLM to flip an incorrect response to a correct response.
    \item As as extreme example, we could assume $\E[A \mid R = 1, B = 1] = 1$, meaning the LLM never flips from right to wrong as long as the correct answer is retained.
    \item We could treat the two cases $\Pb(B = 0) > \Pb(B = 1)$ vs. $\Pb(B = 1) > \Pb(B = 0)$ separately.
\end{enumerate}

As an example, continuing from \eqref{eq:accuracy_derivation1} above, we have that this quantity is greater than $\E[B]$ (the post-CROQ accuracy) iff
\begin{align}
    \E[A \mid B = 0, R = 1]\Pb(R = 1 \mid B = 0) > \Pb(B = 1)\large\{1 &+ \E[A \mid B = 0, R = 1]\Pb(R = 1 \mid B = 0) \\
    &- \E[A \mid B = 1, R = 1]\Pb(R = 1 \mid B = 1) \large\} \label{eq:accuracy_derivation2}
\end{align}
If we use assumptions 1 and 3 from the list above, then we have that the RHS is less than $\Pb(B = 1)$, so we have
\begin{align*}
     \E[A \mid B = 0, R = 1]\Pb(R = 1 \mid B = 0) > \Pb(B = 1) \implies \E[A] > \E[B].
\end{align*}
We could also rewrite this as
\begin{align*}
     \E[A \mid B = 0, R = 1] > \frac{\Pb(B = 1)}{\Pb(R = 1 \mid B = 0)} \implies \E[A] > \E[B].
\end{align*}
In other words, it suffices to raise the accuracy by some multiple of the pre-CROQ accuracy $\Pb(B = 1)$, where this multiple is determined by how often we retain the correct answer when the LLM is wrong. (This is sufficient but not necessary, so it's a conservative standard.)

If we make assumptions 2 and 4 instead of 1 and 3, then from \eqref{eq:accuracy_derivation1} we have that $\E[A] > \E[B]$ iff
\begin{align*}
    \E[A \mid B = 0, R = 1]\Pb(R = 1 \mid B = 0)\Pb(B = 0) > 0
\end{align*}
meaning that as long as we flip some answers from wrong to right, we're guaranteed to improve the accuracy (obviously).
